# Supplementary material for: Higher-order topological phases on fractal lattices
Source: arXiv:2109.03231 ancillary file (2022-05-31)
Supplement: Supplementary file 1 [file Supplementary_FractalHOT.pdf]

# Supplementary Material: Higher-order topological phases on fractal lattices

Sourav Manna,[1,2] Snehasish Nandy,[3] and Bitan Roy[4]

[1] *Department of Condensed Matter Physics, Weizmann Institute of Science, Rehovot 7610001, Israel*
[2] *Max-Planck-Institut für Physik komplexer Systeme, Nöthnitzer Str. 38, 01187 Dresden, Germany*
[3] *Department of Physics, University of Virginia, Charlottesville, Virginia, 22904, USA*
[4] *Department of Physics, Lehigh University, Bethlehem, Pennsylvania, 18015, USA*
(Dated: May 18, 2022)

The Supplementary Materials contain (a) computation of the fractal dimension and generation number [Sec. S1], (b) key details for the derivation of the real space hopping Hamiltonian [Sec. S2], (c) numerical results related to higher-order topological (HOT) insulators on glued Sierpinski triangle fractal [Sec. S3], (d) all numerical analyses of HOT superconductors on Siperpinski carpet and glued Sierpinski triangle fractals [Sec. S4], and (e) additional numerical results [Sec. S5].

## S1. FRACTAL DIMENSION ($d_{\rm frac}$) AND GENERATION NUMBER ($f$)

In the main manuscript we quoted the fractal dimensions ($d_{\rm frac}$) for (a) Sierpinski carpet fractal and (b) glued Sierpinski triangle fractal. Here we show the explicit computation of their fractal dimensions.

**Sierpinski carpet**. This fractal lattice is constructed from a square as follows. We divide the square into $3 \times 3$ squares and place one lattice site at the center of each of the nine squares. Then the square in the middle is removed together with the lattice sites contained in it. We repeat the procedure recursively for each of the eight remaining squares to obtain different generations ($f$). In the $n$th generation the total number of squares is $9^n$ and the total number of unremoved squares is $8^n$. Hence the Sierpinski carpet fractal lattice has a fractal dimension

$$d_{\rm frac} = \frac{\ln 8^n}{\ln \sqrt{9^n}} \approx 1.89. \tag{S1}$$

The Sierpinski carpet fractal lattice of second, third and fourth generations are shown in Fig. S1 (top panel).

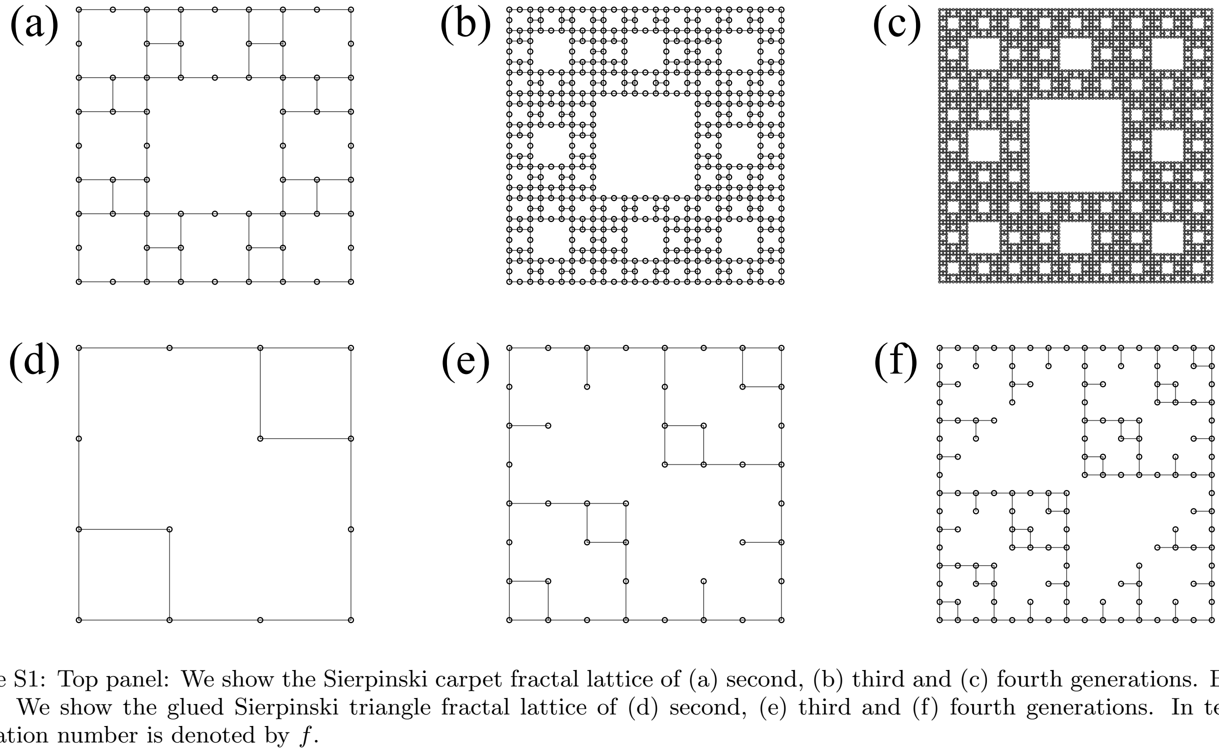


Figure S1: Top panel: We show the Sierpinski carpet fractal lattice of (a) second, (b) third and (c) fourth generations. Bottom panel: We show the glued Sierpinski triangle fractal lattice of (d) second, (e) third and (f) fourth generations. In text the generation number is denoted by $f$.

| Symmetry analyses in Brillouin zone (BZ) | | | | | Symmetry analyses in real space (RS) | | | | |
|---|---|---|---|---|---|---|---|---|---|
| Function | $R^{\rm BZ}_{\pi/2}$ | $R^{\rm BZ}_x$ | $R^{\rm BZ}_y$ | $\mathcal{K}$ | Function | $R^{\rm RS}_{\pi/2}$ | $R^{\rm RS}_x$ | $R^{\rm RS}_y$ | $\mathcal{K}$ |
| $\sin k_x$ | $-\sin k_y$ | $\sin k_x$ | $-\sin k_x$ | - | $i\cos\phi_{jk}$ | $-i\sin\phi_{jk}$ | $i\cos\phi_{jk}$ | $-i\cos\phi_{jk}$ | - |
| $\sin k_y$ | $\sin k_x$ | $-\sin k_y$ | $\sin k_y$ | - | $i\sin\phi_{jk}$ | $i\cos\phi_{jk}$ | $-i\sin\phi_{jk}$ | $i\sin\phi_{jk}$ | - |
| $\cos k_x+\cos k_y$ | $\cos k_x+\cos k_y$ | $\cos k_x+\cos k_y$ | $\cos k_x+\cos k_y$ | + | $C$ | $C$ | $C$ | $C$ | + |
| $m_0$ | $m_0$ | $m_0$ | $m_0$ | + | $m_0$ | $m_0$ | $m_0$ | $m_0$ | + |
| $\cos k_x-\cos k_y$ | $-(\cos k_x-\cos k_y)$ | $\cos k_x-\cos k_y$ | $\cos k_x-\cos k_y$ | + | $\cos 2\phi_{jk}$ | $-\cos 2\phi_{jk}$ | $\cos 2\phi_{jk}$ | $\cos 2\phi_{jk}$ | + |

Table S1: Symmetry analyses of various terms appearing in the momentum space (first five columns) and real sapce (last five columns) Hamiltonian, respectively appearing in Eq. (1) and Eq. (5) of the main text. Terms transforming identically under all symmetry transformations appear in the same row. Here $R^{\rm BZ}_{\pi/2}$ represents a rotation by $\pi/2$ about the $z$ direction under which $\boldsymbol{k}\to(-k_y,k_x)$, while $R^{\rm BZ}_x$ corresponds to the reflection about the $x$ axis under which $\boldsymbol{k}\to(k_x,-k_y)$, and finally $R^{\rm BZ}_y$ stands for the reflection about the $y$ axis under which $\boldsymbol{k}\to(-k_x,k_y)$. On the other hand, $R^{\rm BZ}_{\pi/2}$ represents a rotation by $\pi/2$ about the $z$ direction in the real space under which $\phi_{jk}\to\phi_{jk}+\pi/2$, $R^{\rm RS}_x$ corresponds to the reflection about the $x$ axis in the real space under which $\phi_{jk}\to 2\pi-\phi_{jk}$, and $R^{\rm RS}_y$ corresponds to the reflection about the $y$ axis in the real space under which $\phi_{jk}\to\pi-\phi_{jk}$. Here $m_0$ and $C$ are *real* constants, $\boldsymbol{k}=(k_x,k_y)$ is the momentum, and $\phi_{jk}$ is the azimuthal angle between sites $j$ and $k$, measured about the horizontal direction. We also summarize the transformation of each term under complex conjugation ($\mathcal{K}$), with $\mathcal{K}\boldsymbol{k}\to-\boldsymbol{k}$. In the fifth and tenth columns $+$ $(-)$ corresponds to even (odd).

**Glued Sierpinski triangle**. Firstly we construct the right angle Sierpinski triangle fractal lattice as follows. We start with a right angle triangle and divide it into four equilateral triangles. We place one lattice site at each of the vertices of the right angle triangle and one lattice site at the middle. Then we remove the middle triangle with its lattice site. Now the glued Sierpinski triangle fractal lattice is constructed from a right angle Sierpinski triangle fractal lattice as follows. We glue two right angle Sierpinski triangle fractal lattice along thier hypotenuse and eliminate the common lattice sites. We repeat the procedure recursively for each of the six remaining equilateral triangles to have different generations ($f$). In the $n$th generation the total number of equilateral triangles is $8^n$ and the total number of unremoved equilateral triangles is $6^n$. Hence the Sierpinski carpet fractal lattice has a fractal dimension

$$d_{\rm frac}=\frac{\ln 6^n}{\ln\sqrt{8^n}}\approx 1.72. \tag{S2}$$

We show such fracal lattice of second, third and fourth generations in Fig. S1 (bottom panel).

## S2. DERIVATION OF REAL SPACE HAMILTONIAN

In this section of the Supplementary Materials (SM), we show how to arrive at the real space hopping Hamiltonian for second-order topological insualtor [Eq. (2) of the main manuscript] from the model written in the momentum space [Eq. (1) of the main text]. First we seek the transformation of each term appearing in Eq. (1) of the main text under various symmetry operations. Subsequently, corresponding to each such term, we search for the real space term that transforms identically under all symmetry operations. This analysis is shown in Table S1. Once such one-to-one correspondence is established, we replace each momentum dependent term by its symmetry analog term in the real space, which ultimately leads us to Eq. (2) of the main text.

## S3. NUMERICAL RESULTS FOR HOT INSULATORS ON GLUED SIERPINSKI TRIANGLE FRACTAL

In the main manuscript, we discussed the realization of second-order topological insulators on glued Sierpinski triangle fractals. In particular, we have shown (a) the energy spectra and the local density of states (LDOS) associated with the near (due to finite system size) zero energy modes in systems with both open and periodic boundary conditions [Fig. 3], (b) scaling of the fraction of the origin choices ($F_r$) for which we find quantized quadrupole moment $Q_{xy}=0.5$ (modulo 1) that corroborates the existence of zero energy modes at the outer (predominantly) as well as inner naked (subdominantly) corners with the generation number ($f$) and number of lattice sites ($N$) [Fig. 2(b)], and (c) scaling of the gap ($E_g$) between the zero energy corner modes and closest to zero energy modes that are not corner localized,

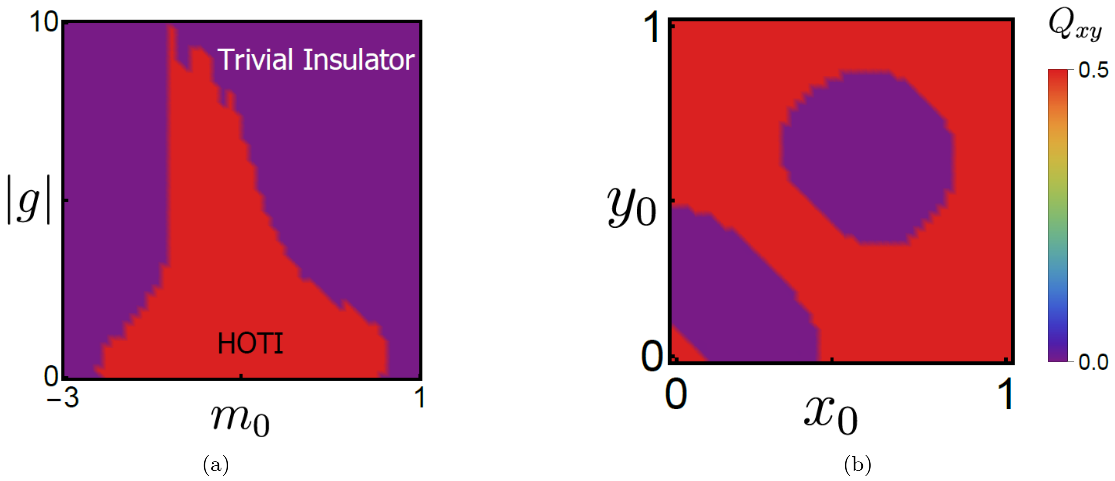


Figure S2: (a) Phase diagram in the $(m_0, |g|)$ plane on glued Sierpinski triangle fractal for $t = t_0 = 1$, $m_0 = 0$ and $g = \sqrt{2}$ showing two distinct phases: (1) a HOT insulator, where $Q_{xy} = 0.5$ and (2) a trivial insulator with $Q_{xy} = 0$. In the entire HOT insulator phase the system supports zero energy outer and naked inner corner modes, when we implement an open boundary condition. (b) Origin $(x_0, y_0)$ dependence of the quadrupole moment $Q_{xy}$ (modulo 1) of a HOT insulator supporting outer and inner naked corner modes [see Fig. 3 of the main manuscript] on glued Sierpinski triangle fractal with open boundary condition. Here $x_0$ and $y_0$ are measured in units of $L$, the linear dimension of the system in each direction. For a majority of the origin choices (approximately 70%) we indeed find $Q_{xy} = 0.5$, corroborating the higher-order bulk-boundary correspondence. Here the results are obtained on glued Sierpinski triangle fractal of generation $f = 6$, containing 1394 sites.

showing that this gap saturates to a finite value as we approach the thermodynamic limit, corresponding to $f \to \infty$ or $N \to \infty$ [Fig. 2(d)]. The last observation guarantees that the corner modes on glued Sierpinski triangle fractals always remain well separated from the rest of the spectra that in turn ensures that the corner modes and the HOT insulators are stable in this system. Furthermore, we found that $F_r \to 1$ (admitted slowly in comparison to that in Sierpinski carpet fractal) in the thermodynamic limit [Fig. 2(b)], showing that $Q_{xy}$ serves as an origin independent bonafide order parameter to identify HOT insulator on glued Sierpinski triangle fractals.

In Fig. S2, we present additional numerical results on glued Sierpinski triangle fractal. Namely, we show a global phase diagram in the $(m_0, |g|)$ plane, showing two topologically distinct phases, a HOT insulator with $Q_{xy} = 0.5$ and a normal or trivial insulator with $Q_{xy} = 0$ [see Fig. S2(a)]. This phase diagram is qualitatively similar to the one shown in Fig. 2(a) of the main manuscript for the Sierpinski carpet fractal. We also show the origin dependence of $Q_{xy}$ of a HOT insulator in this system of sixth generation [see Fig. S2(b)]. Even though for a majority of origin choices (approximately 70%) we indeed find $Q_{xy} = 0.5$, the origin dependence is more prominent in comparison to that in Sierpinski carpet fractal (see Fig. 2(c) of the main manuscript). Nonetheless, as we approach the thermodynamic limit the origin dependence of $Q_{xy} = 0.5$ slowly disappears (see Fig. 2(b) of the main manuscript).

## S4. NUMERICAL ANALYSIS FOR FRACTAL HOT SUPERCONDUCTORS

In the main manuscript, we claimed that the energy spectra in the presence of a local second-order topological pairing [see Eq. (6) of the main text] in fractal second-order or quadrupole Dirac materials are qualitatively similar to the ones shown for HOT insulators on both Sierpinski carpet and glued Sierpinski triangle fractals. In addition, the LDOS associated with the near zero energy Majorana modes (specifically their corner localizations) are also similar to that for the zero energy charged corner modes for HOT insulators in these two fractal lattices. Here we substantiate these claims for both Sierpinski carpet fractal [see Fig. S3(a) and (b)] as well as glued Siperpinski triangle fractal [see Fig. S3(c) and (d)].

Superconducting orders in general can be written as

$$\sum_{\mathbf{k}} \Psi_{\mathbf{k}} \hat{M} \Psi_{-\mathbf{k}} + H.c. = \sum_{\mathbf{k}} \Psi_{\mathbf{k},a} \hat{M}_{ab} \Psi_{-\mathbf{k},b} + H.c. = -\sum_{\mathbf{k}} \Psi_{-\mathbf{k},b} \hat{M}_{ab} \Psi_{\mathbf{k},a} + H.c. = -\sum_{\mathbf{k}} \Psi_{-\mathbf{k},b} \hat{M}^{\top}_{ba} \Psi_{\mathbf{k},a} + H.c.$$

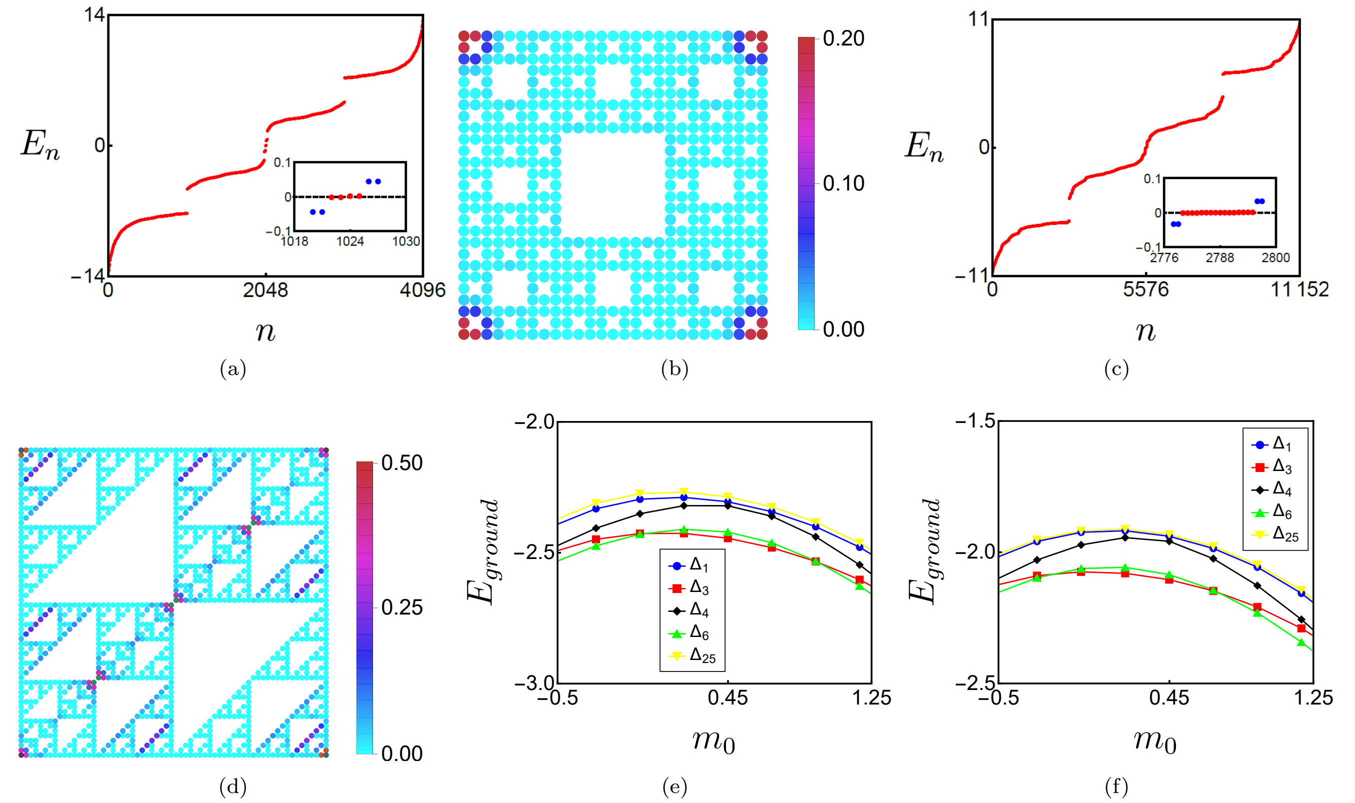


Figure S3: (a) Energy spectra for local second-order pairing ($\Delta_3 = 5.0$) on a Sierpinski carpet fractal of generation $f = 3$ (containing 512 sites) for $t = t_0 = 1$, $m_0 = 3$ and $g = 2$, such that the normal state (with $\Delta_3 = 0$) is a trivial insulator [see Fig. 2(a) of the main text]. (b) Spatial distribution of the local density of states (LDOS) of the four near zero energy modes, shown in red in the inset of (a), confirming their sharp outer corner localization. (c) Energy spectra for local second-order pairing ($\Delta_3 = 4.0$) on a glued Sierpinski triangle fractal of generation $f = 6$ (containing 1394 sites) for $t = t_0 = 1$, $m_0 = 3$ and $g = 2$, such that the normal state (with $\Delta_3 = 0$) is a trivial insulator [see Fig. S2(a)]. (d) Spatial distribution of the LDOS of the sixteen near zero energy modes, shown in red in the inset of (c), confirming their sharp localizations at both outer and inner naked corners. The inner edges making $\pi/4$ angle with the horizon also absorb a tiny fraction of the LDOS, as the insulating second-order Wilson-Dirac mass vanishes in this direction. In (a)-(d), we implement open boundary condition. Comparison of the ground state energy density ($E_{ground}$) of all six local pairings for their equal amplitudes (set to be 1.0) on (e) Sierpinski carpet and (f) glued Sierpinski triangle fractals as a function of $m_0$ with the other parameter values mentioned above. These analyses show that the local second-order pairing ($\Delta_3$) is energetically most favored (possessing the lowest ground state energy density) over a wide range of $m_0$. Thus local second-order pairing can be realized in fractal quadrupole Dirac materials. For notations see Eq. (S4).

$$= -\sum_{\mathbf{k}} \Psi_{\mathbf{k},b} \hat{M}^{\top}_{ba} \Psi_{-\mathbf{k},a} + H.c. = -\sum_{\mathbf{k}} \Psi_{\mathbf{k}} \hat{M}^{\top} \Psi_{-\mathbf{k}} + H.c. \tag{S3}$$

Here $\mathbf{k}$ is the momentum, $\Psi$ is an $n$-component spinor and $\hat{M}$ is an $n \times n$ Hermitian matrix, and H.c. stands for the Hermitian conjugate, where $n$ is an arbitrary integer. Summation over repeated indices is assumed. The above identity holds only if the Hermitian matrix satisfies $\hat{M}^{\top} = -M$, which mandates that $\hat{M}$ must be a purely imaginary Hermitian matrix. While arriving this conclusion, we used $\{\Psi_{\mathbf{k},a}, \Psi_{-\mathbf{k},b}\} = 0$, which indicates the fermionic nature of the quasiparticles, satisfying the Pauli exclusion principle. We follow this guiding principle to identify all the local or onsite pairings, represented by constant or momentum independent $\hat{M}$.

To examine the possibility of realizing the local second-order pairing in a second-order fractal Dirac insulator (either topological or trivial), we compare the ground state energies of all six local superconducting pairings in this system. The corresponding effective single-particle Hamiltonian reads as

$$H^{\text{pairing}}_{\text{effect}} = \Delta_1 \Gamma_{\alpha 22} + \Delta_{25} \left( \frac{\Gamma_{\alpha 32} + \Gamma_{\alpha 01}}{\sqrt{2}} \right) + \Delta_3 \Gamma_{\alpha 12} + \Delta_4 \Gamma_{\alpha 00} + \Delta_6 \Gamma_{\alpha 03}. \tag{S4}$$

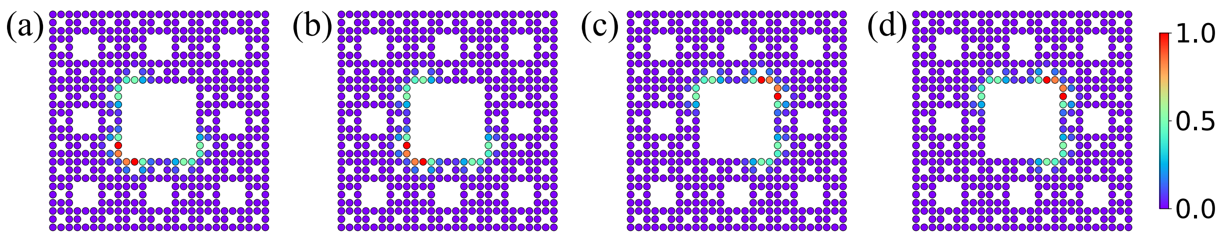


Figure S4: Local density of states associated with four finite (but closest to zero) energy states [shown by blue dots in the inset of Fig. 1(a) of the main text] on a Sierpinski carpter fractal of generation $f = 3$ (containing 512 sites) for $t = t_0 = 1$, $m_0 = 0$ and $g = \sqrt{2}$. They are localized near (but not at) the four innermost corners of the fractal lattice. However, even with increasing generation number they never becomes zero energy modes, as shown in Fig. 2(d) of the main text, as there exists no inner corner with coordination number 2, unlike the outer corners. In each panel, we normalize the local density of states by its maximum value.

Here $\alpha = 1, 2$ reflects the U(1) gauge redundancy in defining the superconducting phase, and without any loss of generality we choose $\alpha = 1$ for our numerical analyses. The eight-dimensional matrices $\Gamma_{\alpha\nu\rho} \equiv \eta_\alpha \sigma_\nu \tau_\rho$. Three sets of the Pauli matrices $\{\eta_\alpha\}$, $\{\sigma_\nu\}$ and $\{\tau_\rho\}$ respectively operate on the Nambu or particle-hole, spin and orbital indices, with $\alpha, \nu, \rho = 0, \cdots, 3$. While arranging the Nambu doubled spinor we absorb the unitary part of the time reversal operator $\Gamma_{20} \equiv \sigma_2 \tau_0$ on the hole part. While the local pairings with amplitudes $\Delta_1$, $\Delta_3$, $\Delta_4$ and $\Delta_6$ transform as singlets, the one with amplitude $\Delta_{25}$ transforms as a doublet (altogether yielding six pairing matrices). Readers can verify that only the $\Delta_3$ pairing meets all the requisite symmetry criteria to represent a local second-order topological pairing, which we discussed in details in the main text, where we set $\Delta_3 \to \Delta$ for notational simplicity. As all these parings are local, they can be implemented on any lattice (like two fractal lattices we considered) as on site terms.

To compare the ground state energies of all the local paired states, we implement them on two fractal lattices and numerically diagonalize the total effective single-particle Nambu Hamiltonian. We set the amplitudes of all the pairings to be equal, and sum over all the negative energy eigenvalues (the filled states at half-filling) and subsequently divide this quantity by $4N$, where $N$ is the number of lattice sites, to obtain the ground state energy density ($E_{ground}$). The results obtained on Sierpinski carpet and glued Sierpinski triangle fractals are respectively shown in Fig. S3(e) and Fig. S3(f). It shows that for a wide range of $m_0$ the local second-order pairing (namley $\Delta_3$) possesses the lowest ground state energy density, and thus can be energetically favored.

## S5. ADDITIONAL NUMERICAL RESULTS

In this section, we present some additional numerical results to further anchor some of our claims from the main manuscript. In Fig. S4, we display the local density to states (LDOS) for four states at finite (but small or close to zero) energy. They are indeed localized near the four innermost corners of the Sierpinski carpet fractal lattice. However, it should be noted that these modes never become zero energy states even as we approach the thermodynamic limit when the generation number $f \to \infty$ or equivalently the number of sites in the fractal lattice $N \to \infty$. This conclusion is substantiated from the the spectral gap ($E_g$) between the zero energy modes [shown by red dots in the inset of Fig. 1(a) of the main text] and the closest to zero energy [shown by blue dots in the inset of Fig. 1(a) of the main text] modes, which saturates to a finite value as $f \to \infty$ or $N \to \infty$. Therefore, we always find only four topological zero energy modes which are highly localized at the outer four corners of the Sierpinski carpet fractal lattice, irrespective of its generation number.

In Fig. S5, we show the LDOS for all sixteen closest to zero energy modes, we found on glued Sierpinski triangle fractal lattice of generation number $f = 6$ containing 1394 sites [see Fig. 3 of the main manuscript]. Notice that at least a fraction of the total LDOS for each such mode is localized at the inner edges or corners of such fractal lattice, besides at four outer corners, when we implement open boundary condition in the system. As a consequence of such fragmented LDOS of the topological zero energy modes among the outer corners and inner boundaries of glued Sierpinski triangle fractal, when we impose periodic boundary condition in this system, the number of zero energy modes do not change. Only their entire spectral weight shifts to the inner boundaries, as claimed in the main manuscript. This outcome is in stark contradiction with the situation on Sierpinski carpet fractal, where the LDOS of

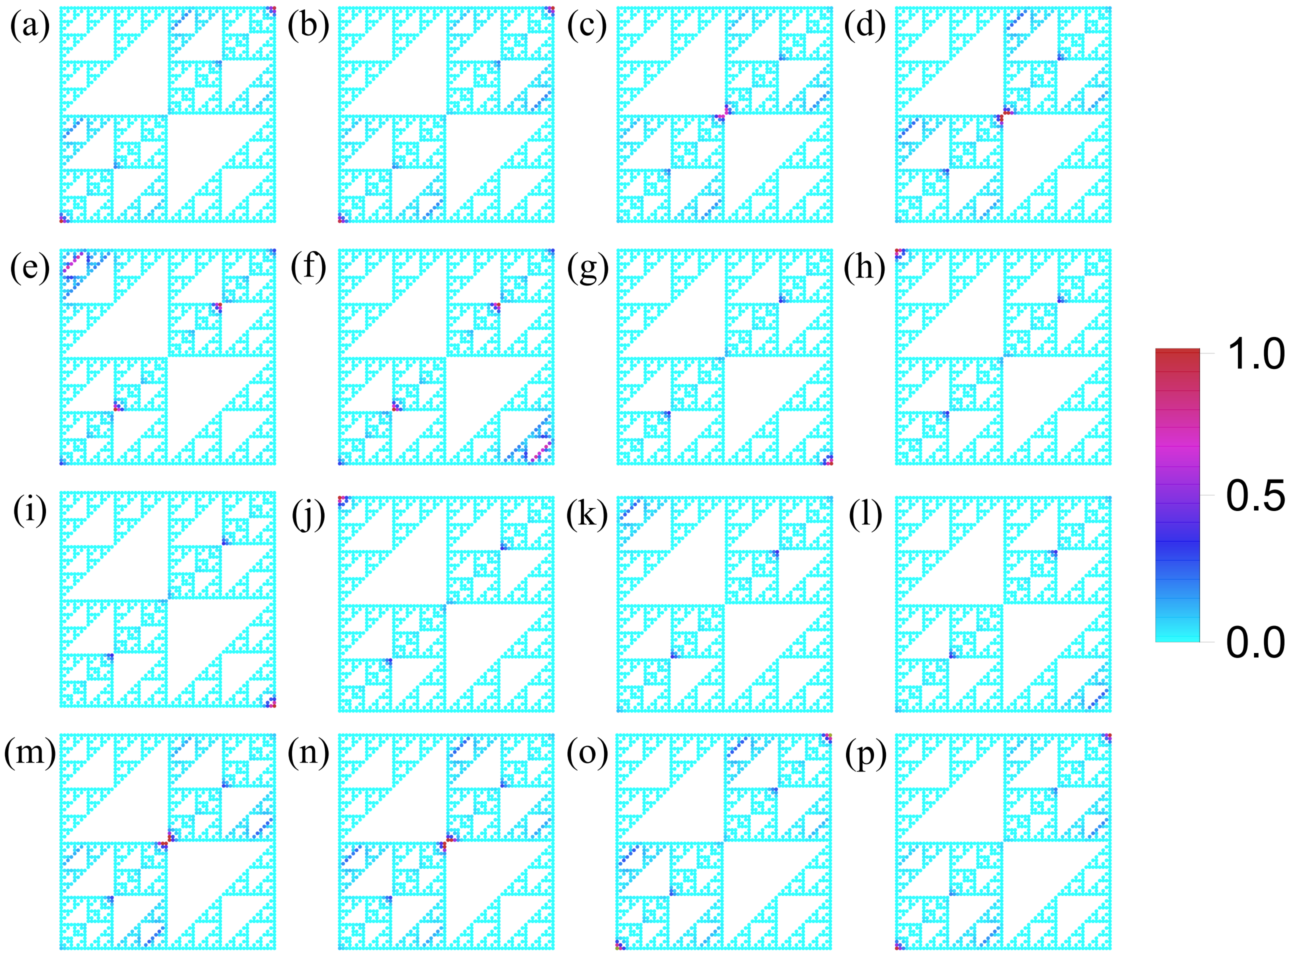


Figure S5: Local density of states for all sixteen zero energy modes on glued Sierpinski triangle fractal of sixth generation ($f = 6$) containing 1394 sites for $t = t_0 = 1$, $m_0 = 0$ and $g = \sqrt{2}$ with open boundary condition. Notice that within such zero-energy manifold there exists no state which is exclusively localized at the outer corners. As a result when we impose a periodic boundary condition, the number of zero energy modes does not change. Only their entire weight shifts to the inner corners. In each panel, we normalize the local density of states by its maximum value.

four zero energy modes are highly localized at four outer corners of the lattice. As a result when we impose periodic boundary condition on this system, there is no zero energy mode localized at inner corners. Recall that the modes localized near inner corners are always at small, but finite energy.
